# Supplementary material for: Momentum-based Weight Interpolation of Strong Zero-Shot Models for Continual Learning
Source: arXiv:2211.03186 source file (2022-11-06)
Supplement: Supplementary file 1 [file supplementary.tex]

\begin{centering}
\section*{\Large{Supplementary:  Integrating Language Guidance into Vision-based Deep Metric Learning}}
\end{centering}
\vspace{12pt}

\setcounter{equation}{0}
\setcounter{figure}{0}
\setcounter{table}{0}
\setcounter{page}{1}
\makeatletter

\appendix
\section{Experimental Details}
\label{supp:sec:exp_details}
For all our experiments, we utilize PyTorch \cite{pytorch}. Underlying backbones and training protocols are adapted from previous research (e.g. \cite{roth2020revisiting,musgrave2020metric,softriple,multisimilarity,milbich2020diva,s2sd}) including the codebase provided through \cite{roth2020revisiting}. More specifically, our experiments utilize either a ResNet50 \cite{resnet} with embedding dimensionality of 128 or 512 as well as an Inception-BN \cite{inceptionv1} with dimensionality 512. The ImageNet-pretrained network weights were taken from \texttt{timm} \cite{rw2019timm} as well as \texttt{torchvision} \cite{pytorch}.

Both for studies of relative improvements as well as state-of-the-art performance comparisons, optimization is done using Adam \cite{adam} with a base learning rate of $10^{-5}$, consistent weight decay \cite{weight_decay} of $3\cdot 10^{-4}$ and batchsizes between 80 and 112. Our relative evaluation follows the protocol proposed in \cite{roth2020revisiting}, while for our state-of-the-art comparison, we provide a thorough evaluation against different literature methods separated by the utilized underlying backbone. For our language backbone, we chose the language-part of CLIP \cite{clip} (specifically the ``ViT-B/32'' variant) and the provided tokenizer, but show in section \ref{subsec:arch_ablations} that essentially any big language model can be used for this task. This shows that improvements are not based on potential minor dataset overlap in the image-part of the CLIP training protocol and potential implicit information bleeding into the language model. We also note that the authors of \cite{clip} themselves highlight that even with data overlap, performance is not impacted in a relevant fashion. Applying language-guidance to S2SD \cite{s2sd}, we found placing more emphasis on the feature distillation part instead of the dimensionality distillation worked better in conjunction with both \textit{ELG} and \textit{PLG}. To avoid large-scale hyperparameter grid searches, we thus simply set the weights for dimensionality matching to zero and only adjust the feature distillation weight.

For the scaling $\omega$ of our language-guidance (see Eq. \ref{eq:final_eq}), we found $\omega\in[1, 10]$ to work consistently for our experiments on CARS196 and CUB200-2011 and $\omega\in[0.1, 1]$ on Stanford Online Products, which accounts for the magnitude of the base loss function $\mathcal{L}_\text{DML}$. For the state-of-the-art study in \S\ref{subsec:sota}, we found these parameter values to transfer well to the other backbones and embedding dimensionalities.

\section{Additional Experimental Results}
\label{supp:sec:experiments}
\subsection{Additional language models}
\label{supp:subsec:languagemodels}
To study the impact of language guidance provided with different pretrained language models, Table \ref{supp:tab:choice_of_language_models} provides an extensive evaluation of different language model architectures and pretrainings. As can be seen, performance boosts are consistent, regardless of the exact choice of language model, supporting the general benefit of language as an auxiliary, performance-facilitating modality for finegrained visual similarity tasks.

\subsection{Conceptual approaches to language inclusion}
\label{supp:subsec:concepts}
\begin{table*}[t]
    \caption{\textit{Relative comparison.} We follow protocols proposed in \cite{roth2020revisiting}\protect\footnotemark, with no learning rate scheduling, to ensure exact comparability. The results show significant improvements on CUB200 and CARS196 when language-guidance is applied (with expert- and pseudolabels). ($^*$) For SOP, only 12 superlabels are given for 11,318 training classes. Similarly, SOP only contains very few samples per class, making pseudolabel class estimates very noisy. This makes the benefits of language guidance limited.}
\vspace{-5pt}    
 \footnotesize
  \setlength\tabcolsep{1.4pt}
  \centering
  %\begin{tabular}{l|c|ccc|c}
  \resizebox{0.95\textwidth}{!}{
  \begin{tabular}{l || c | c | c || c | c| c || c | c | c}
     \toprule
     \multicolumn{1}{l}{\textsc{Benchmarks}$\rightarrow$} & \multicolumn{3}{c}{\textsc{CUB200-2011}} & \multicolumn{3}{c}{\textsc{CARS196}} & \multicolumn{3}{c}{\textsc{SOP}($^*$)} \\
     \midrule
     \textsc{Approaches} $\downarrow$ & R@1 & NMI & mAP@1000 & R@1 & NMI & mAP@1000 & R@1 & NMI & mAP@1000\\
    \midrule
    \rowcolor{vvlightgray} 
    \textbf{Multisimilarity} & 62.8 $\pm$ 0.2 & 67.8 $\pm$ 0.4 & 31.1 $\pm$ 0.3 & 81.6 $\pm$ 0.3 & 69.6 $\pm$ 0.5 & 31.7 $\pm$ 0.1 & 76.0 $\pm$ 0.1  & 89.4 $\pm$ 0.1  & 43.3 $\pm$ 0.1 \\
    \hline
    +\textit{ELG} & 67.3 $\pm$ 0.2 & 69.6 $\pm$ 0.6 & 34.8 $\pm$ 0.2 & 85.3 $\pm$ 0.1 & 71.7 $\pm$ 0.2 & 32.7 $\pm$ 0.2 & 76.0 $\pm$ 0.2  & 89.5 $\pm$ 0.1  & 43.5 $\pm$ 0.1 \\ 
    % +\textit{PLG} Top-1 & 66.2 $\pm$ 0.6 & 68.4 $\pm$ 0.3 & 33.8 $\pm$ 0.2 & 85.2 $\pm$ 0.1 & 71.1 $\pm$ 0.3 & 32.7 $\pm$ 0.1 & 76.1 $\pm$ 0.2  & 89.4 $\pm$ 0.2  & 43.4 $\pm$ 0.1 \\ 
    +\textit{PLG} Top-5 & 67.1 $\pm$ 0.4 & 69.6 $\pm$ 0.6 & 34.6 $\pm$ 0.5 & 85.4 $\pm$ 0.2 & 71.3 $\pm$ 0.1 & 32.8 $\pm$ 0.2 & 76.4 $\pm$ 0.1  & 89.6 $\pm$ 0.1  & 43.7 $\pm$ 0.1 \\ 
    % +\textit{PLG} Top-5 No Mask &&&&&&&&&\\
    \midrule 
    \rowcolor{vvlightgray} 
    \textbf{Margin}, $\beta=1.2$ & 62.7 $\pm$ 0.6 & 68.0 $\pm$ 0.3 & 32.2 $\pm$ 0.3 & 79.4 $\pm$ 0.5 & 66.6 $\pm$ 0.7 & 32.8 $\pm$ 0.2 & 78.0 $\pm$ 0.3  & 90.3 $\pm$ 0.2  & 46.3 $\pm$ 0.2 \\ 
    \hline
    +\textit{ELG} & 65.3 $\pm$ 0.5 & 68.5 $\pm$ 0.4 & 33.5 $\pm$ 0.3 & 83.2 $\pm$ 0.5 & 69.0 $\pm$ 0.6 & 33.4 $\pm$ 0.3 & 77.8 $\pm$ 0.1  & 90.2 $\pm$ 0.1  & 46.1 $\pm$ 0.1 \\ 
    % +\textit{PLG} Top-1 & 64.9 $\pm$ 0.4 & 68.4 $\pm$ 0.4 & 33.0 $\pm$ 0.3 & 83.2 $\pm$ 0.4 & 68.7 $\pm$ 0.7 & 33.5 $\pm$ 0.3 & 78.1 $\pm$ 0.2  & 90.2 $\pm$ 0.3  & 46.3 $\pm$ 0.1 \\ 
    +\textit{PLG} Top-5 & 65.2 $\pm$ 0.5 & 68.5 $\pm$ 0.4 & 33.5 $\pm$ 0.3 & 83.4 $\pm$ 0.4 & 69.1 $\pm$ 0.4 & 33.7 $\pm$ 0.3 & 78.3 $\pm$ 0.2  & 90.3 $\pm$ 0.2  & 46.5 $\pm$ 0.1 \\ 
    \midrule 
    \rowcolor{vvlightgray} 
    \textbf{Multisimilarity + S2SD} & 67.7 $\pm$ 0.3 & 71.5 $\pm$ 0.2 & 35.5 $\pm$ 0.2 & 86.5 $\pm$ 0.1 & 71.4 $\pm$ 0.4 & 35.1 $\pm$ 0.3 & 77.7 $\pm$ 0.2  & 89.9 $\pm$ 0.1  & 45.3 $\pm$ 0.3 \\ 
    \hline
    +\textit{ELG} & 68.9 $\pm$ 0.4 & 72.5 $\pm$ 0.3 & 36.4 $\pm$ 0.5 & 88.2 $\pm$ 0.2 & 72.0 $\pm$ 0.1 & 36.0 $\pm$ 0.1 & 77.8 $\pm$ 0.1  & 90.0 $\pm$ 0.2  & 45.3 $\pm$ 0.2 \\ 
    % +\textit{PLG} Top-1 & 68.7 $\pm$ 0.4 & 72.4 $\pm$ 0.4 & 36.2 $\pm$ 0.5 & 88.4 $\pm$ 0.2 & 72.4 $\pm$ 0.3 & 36.2 $\pm$ 0.2 & 77.9 $\pm$ 0.2  & 90.0 $\pm$ 0.2  & 45.4 $\pm$ 0.2 \\ 
    +\textit{PLG} Top-5 & 69.0 $\pm$ 0.4 & 72.4 $\pm$ 0.2 & 36.6 $\pm$ 0.3 & 88.4 $\pm$ 0.3 & 72.4 $\pm$ 0.2 & 36.2 $\pm$ 0.2 & 78.0 $\pm$ 0.1  & 90.0 $\pm$ 0.1  & 45.6 $\pm$ 0.1 \\ 
    \bottomrule 

    \end{tabular}}
    \label{tab:supp_relative_results}
 \end{table*}

\begin{table}[h!]
    \caption{\textit{Models vs. guidance quality.} Performance improves regardless of the exact large pretrained language model. Strong improvements can even be achieved through large-scale pretrained word embeddings such as FastText \cite{fasttext} and GloVe \cite{glove}. However, using less transferable word hierarchies falls short in comparison.}
 \footnotesize
  \setlength\tabcolsep{1.4pt}
  \centering
  %\begin{tabular}{l|c|ccc|c}
  \begin{tabular}{l || c | c || c | c }
     \toprule
     \multicolumn{1}{l}{\textsc{Benchmarks}$\rightarrow$} & \multicolumn{2}{c}{\textsc{CUB200-2011}} & \multicolumn{2}{c}{\textsc{CARS196}} \\
     \midrule
     \multirow{2}{*}{\textsc{Models} $\downarrow$} & \multirow{2}{*}{R@1} & mAP & \multirow{2}{*}{R@1} & mAP\\
      &  & @1000 & & @1000\\
    \midrule
    \rowcolor{vlightgray}
    \textbf{Baseline} & 62.8 $\pm$ 0.2 & 31.1 $\pm$ 0.3 & 81.6 $\pm$ 0.3 & 31.7 $\pm$ 0.1\\ 
    \rowcolor{vvlightgray}    
    + CLIP-L \cite{clip} & 67.3 $\pm$ 0.2 & \textbf{34.8 $\pm$ 0.2} & 85.3 $\pm$ 0.1 & \textbf{32.7 $\pm$ 0.2} \\
    % \hline
    % + $\mathbb{S}^{N-1}\left(\mathcal{N}(0,1)\right)$ & - $\pm$ - & - $\pm$ - & - $\pm$ - & - $\pm$ -\\
    \midrule        
    \multicolumn{5}{>{\columncolor[gray]{.9}}l}{\textbf{(a) Language Models}} \\
    \hline
    + BERT \cite{bert} & 66.9 $\pm$ 0.3 & 33.5 $\pm$ 0.2 & 84.9 $\pm$ 0.1 & 32.3 $\pm$ 0.1\\
    + DistBert \cite{distilbert} & 66.7 $\pm$ 0.1 & 33.4 $\pm$ 0.2 & 85.4 $\pm$ 0.4 & 32.4 $\pm$ 0.1\\    
    + Roberta-B \cite{roberta} & 67.0 $\pm$ 0.2 & 33.8 $\pm$ 0.2 & 84.9 $\pm$ 0.1 & 32.3 $\pm$ 0.3\\
    + Roberta-L \cite{roberta} & 67.3 $\pm$ 0.2 & 33.9 $\pm$ 0.3 & 85.1 $\pm$ 0.2 & 32.4 $\pm$ 0.2\\
    + DistRoberta \cite{huggingface} & 66.0 $\pm$ 0.2 & 32.2 $\pm$ 0.2 & 85.0 $\pm$ 0.3 & 32.1 $\pm$ 0.2\\
    + Reformer \cite{Kitaev2020Reformer} & 66.7 $\pm$ 0.1 & 33.1 $\pm$ 0.1 & 85.5 $\pm$ 0.2 & 32.0 $\pm$ 0.2\\
    + MPNet \cite{mpnet} & 66.2 $\pm$ 0.3 & 32.3 $\pm$ 0.2 & 85.4 $\pm$ 0.2 & 32.3 $\pm$ 0.3\\
    + GPT2 \cite{gpt2} & 67.0 $\pm$ 0.3 & 33.7 $\pm$ 0.1 & 84.8 $\pm$ 0.4 & 32.4 $\pm$ 0.1\\
    \hline
    + Top 3 & \textbf{67.5 $\pm$ 0.2} & 34.5 $\pm$ 0.3 & \textbf{85.6 $\pm$ 0.3} & 32.5 $\pm$ 0.3\\   
    \bottomrule
    \end{tabular}
    \label{supp:tab:choice_of_language_models}
 \end{table}
\begin{figure}[h!]
    \centering
    \includegraphics[width=0.48\textwidth]{images/conv.png}
    \caption{\textit{Impact on convergence.} Matching performance is reached much earlier, with significantly better overall downstream generalization performance.
    %. Visualization is capped at 100 epochs for qualitative comparability.
    }
    \label{fig:convergence}
\end{figure}
To directly incorporate language context into a discriminative DML objective, we utilize the language similarities to either adjust the mining mask or the loss scale in the multisimilarity loss \cite{multisimilarity}. To adjust the mining mask, given an anchor sample $x_a$, positives $x_p$ and negatives $x_n$ are selected if, respectively,
\begin{equation}
\begin{split}
    f\left(S^\text{lang}_{a, p}, s(\psi, \psi_p)\right) &< \min_{\psi_k \in \mathcal{B}, y_k \neq y_a} s(\psi_a, \psi_k) + \epsilon\\
    f\left(S^\text{lang}_{a, n}, s(\psi_a, \psi_n)\right) &< \min_{\psi_k \in \mathcal{B}, y_k = y_a} s(\psi_a, \psi_k) - \epsilon
\end{split}
\end{equation}
with similarity function $s(\bullet, \bullet)$ and language similarity scaling $f(\bullet, \bullet)$. For $f(\bullet, \bullet)$, we investigate different orders of interpolation 
\begin{equation}
f(S^\text{lang}_{ij}, S^\text{img}_{ij})_{\nu_1, \nu_2} = \left[(1 - \nu_1) \cdot {S^\text{lang}_{ij}}^{\nu_2} + \nu_1 \cdot {S^\text{img}_{ij}}^{\nu_2}\right]^{1/{\nu_2}}
\end{equation}
to adjust between sole visual similarity and language similarity.
To re-weight loss components (with positive and negative pairs for anchor $x_a$, $\mathcal{P}^+_a$ and $\mathcal{P}^-_a$), we instead compute
\begin{equation}
\begin{split}
    \mathcal{L}^\textit{ELG}_\text{MSIM} &= \frac{1}{|\mathcal{B}|}\sum_{i=1}^{|\mathcal{B}|} \frac{1}{\alpha}\log\left( 1 + \sum_{k\in\mathcal{P}^+_i} e^{-\alpha\left(\frac{S^\text{lang}_{ik}}{S^\text{img}_{ik}}\right)^{\nu_3}(S^\text{img}_{ik} - \lambda)} \right)\\  
    &+ \frac{1}{\beta} \log\left( 1 + \sum_{k\in\mathcal{P}^-_i} e^{\beta\left(\frac{S^\text{lang}_{ik}}{S^\text{img}_{ik}}\right)^{\nu_4}(S^\text{img}_{ik}-\lambda)} \right)
\end{split}
\end{equation}
thus providing a scaling to the utilized visual similarity $S^\text{img}_{ik}$ based on the (relative) similarity to the respective language similarity.
In all cases, a grid search both over newly introduced hyperparameters ($\nu_1$, $\nu_2$, $\nu_3$ and $\nu_4$) as well as the default multisimilarity loss parameters ($\alpha, \beta, \lambda$) is performed.
For the language similarity scaling $f(\bullet, \bullet)$, we found linear interpolation ($\nu_1 = \nu_2 = 1$) to work best. For $\mathcal{L}^\textit{ELG}_\text{MSIM}$, we found $\nu_3 = \nu_4 = 0.75$ to work well, but had to readjust $\alpha=1.5$ and $\beta=45$ slightly to account for the change in magnitude.

For our matching objective, in which we incorporate language context by training either a MLP over embeddings or a transformer (ViT, \cite{vit}) over a sequence of network features to predict language embeddings $\psi_\text{lang}$, the respective networks are trained following  
\begin{equation}
    \mathcal{L}_\text{Match}(\psi_i, \phi_i, \psi_{\text{lang}, i}) = g_\rho^\text{match}(\psi_i, \phi_i)^T\psi_{\text{lang}, i}
\end{equation}
with $g_\rho^\text{match}(\psi_i, \phi_i)$ denoting the unit-normalized mapping from embedding/feature space to (normalized) language space using either the MLP or ViT with parameters $\rho$.

Finally, as a base reference, we also investigate CLIP-style training in which we utilize direct contrastive training between image and language embeddings following \cite{clip} as regularizer against $\mathcal{L}_\text{DML}$:
\begin{equation}
\begin{split}
    \mathcal{L}_\text{CLIP}(S^\text{mixed}) &= \frac{1}{|\mathcal{B}|}\sum_{i}^{|\mathcal{B}|}-\frac{1}{2}\log\left(\sigma\left(S^\text{mixed}_{i,:}\cdot e^T\right)_i\right)\\ &-\frac{1}{2}\log\left(\sigma\left(S^\text{mixed}_{:,i}\cdot e^T\right)_i\right)
\end{split}
\end{equation}
with similarity matrix between minibatch image and language embeddings $S^\text{mixed}$.

%%%%%%%%%%%%%%
\subsection{Language guidance from pseudolabels}
\label{supp:subsec:plangg_ablations}
\begin{table}[h!]
\caption{\textit{Ablations on Pseudolabel guidance.} More pseudolabels per class improve generalization performance, with class-level pseudolabelling and distillation from a single average language similarity matrix offering highest improvements.}
\footnotesize
\setlength\tabcolsep{1.4pt}
\centering
%\begin{tabular}{l|c|ccc|c}
\begin{tabular}{l || c | c || c | c }
\toprule
\multicolumn{1}{l}{\textsc{Benchmarks}$\rightarrow$} & \multicolumn{2}{c}{\textsc{CUB200-2011}} & \multicolumn{2}{c}{\textsc{CARS196}} \\
\midrule
\multirow{2}{*}{\textsc{Approaches} $\downarrow$} & \multirow{2}{*}{R@1} & mAP & \multirow{2}{*}{R@1} & mAP\\
&  & @1000 & & @1000\\
\midrule
\rowcolor{vlightgray}
Baseline & 62.8 $\pm$ 0.2 & 31.1 $\pm$ 0.2 & 81.6 $\pm$ 0.3 & 31.7 $\pm$ 0.1 \\
\rowcolor{vvlightgray}    
+ \textit{ELG} & 67.3 $\pm$ 0.2 & 34.8 $\pm$ 0.2 & 85.3 $\pm$ 0.1 & 32.7 $\pm$ 0.2 \\
\midrule
\multicolumn{5}{>{\columncolor[gray]{.9}}l}{\textbf{Number of pseudolabels}} \\
\hline
+ \textit{PLG} & 66.2 $\pm$ 0.6 & 33.8 $\pm$ 0.2 & 85.2 $\pm$ 0.1 & 32.7 $\pm$ 0.1 \\    
% + \textit{plangg} (Top-2) & 66.6 $\pm$ 0.3 & 34.1 $\pm$ 0.2 & 85.2 $\pm$ 0.2 & 32.6 $\pm$ 0.1 \\   
+ \textit{PLG} (Top-5) & 67.1 $\pm$ 0.4 & 34.6 $\pm$ 0.5 & 85.4 $\pm$ 0.2 & 32.8 $\pm$ 0.2 \\   
+ \textit{PLG} (Top-10) & 67.2 $\pm$ 0.2 & 34.5 $\pm$ 0.3 & 85.3 $\pm$ 0.2 & 32.4 $\pm$ 0.3 \\   
+ \textit{PLG} (Top-20) & 67.0 $\pm$ 0.1 & 34.5 $\pm$ 0.2 & 84.9 $\pm$ 0.4 & 32.1 $\pm$ 0.3 \\   
\midrule
\multicolumn{5}{>{\columncolor[gray]{.9}}l}{\textbf{Word Hierarchies}} \\
\textit{PLG}+WordNet (Top-5) & 64.4 $\pm$ 0.1 & 31.5 $\pm$ 0.2 & 82.9 $\pm$ 0.2 & 31.3 $\pm$ 0.2\\
\textit{pseudo}-HierMatch & 65.0 $\pm$ 0.2 & 32.3 $\pm$ 0.2 & 82.8 $\pm$ 0.3 & 31.6 $\pm$ 0.2\\
\hline
\multicolumn{5}{>{\columncolor[gray]{.9}}l}{\textbf{Different pseudolabel matching methods}} \\
\hline
Sample (Top-5) & 67.0 $\pm$ 0.1 & 34.2 $\pm$ 0.1 & 85.2 $\pm$ 0.2 & 32.2 $\pm$ 0.3 \\   
Dense (Top-5) & 67.0 $\pm$ 0.2 & 33.7 $\pm$ 0.4 & 84.0 $\pm$ 0.1 & 31.5 $\pm$ 0.4 \\   
Multi (Top-5) & 67.2 $\pm$ 0.1 & 34.3 $\pm$ 0.2 & 85.1 $\pm$ 0.2 & 32.2 $\pm$ 0.1 \\   
Dense + Multi & 66.0 $\pm$ 0.3 & 34.1 $\pm$ 0.2 & 84.3 $\pm$ 0.3 & 31.9 $\pm$ 0.2 \\   
\bottomrule
\end{tabular}
\label{tab:plangg_ablations}
\end{table}

% To motivate our proposed state-of-the-art pseudolabel guidance (\S\ref{subsec:language_guided}, 
% Table \ref{tab:sota}), 
For \textit{PLG}, we investigate performance dependence on the number of top-$k$ pseudolabels assigned to every class and their inclusion into training (\S\ref{subsec:language_guided}.
Table \ref{tab:plangg_ablations} highlights that more pseudolabels benefit generalization (optimum for $k\in[5, 10]$), that distillation from a single averaged similarity matrix (see Eq. \ref{eq:multi_match}) performs better than (or comparable to) joint distillation from each pseudolabel similarity matrix (``\textit{Multi (Top-5)}''), and that is does not matter if pseudolabels are computed for classes or individual samples (``\textit{Sample}''). 

In addition, we study whether computing a pseudolabel similarity matrix for each pseudolabel pairing, disregarding the ordering\footnote{E.g. for $k=5$, ``\textit{Dense}'' introduces $k^2 = 25$ target matrices.}, benefits overall performance (``\textit{Dense (Top-5)}'' and ``\textit{Dense + Multi}''), but found no notable benefit. Furthermore, Table \ref{tab:plangg_ablations} shows that leveraging hierarchies as described in \S\ref{subsec:arch_ablations} also performs notable worse in the pseudolabel domain.
%%%%%
Finally, we find impact on overall training time of \textit{PLG} to be negligible, while convergence are in parts even improved (see Supp.-Fig. \ref{fig:convergence}).

\subsection{Convergence of \textit{PLG} models}
Figure \ref{fig:convergence} shows that \textit{PLG (Top-5)} allows underlying objectives to reach similar performance after significantly less training, with much higher overall performance after full training. With \textit{PLG} only requiring an initial forward pass of training samples through the ImageNet-pretrained backbone and of all unique classnames through the language model, impact on overall training time is also negligible.
